# Supplementary material for: GX-Plug: a Middleware for Plugging Accelerators to Distributed Graph Processing
Source: arXiv:2203.13005 source file (2022-03-31)
Supplement: Supplementary file 1 [file SI_SystemVIPC.tex]

\subsection{System V IPC-based Deployment {\color{red} \textbf{\textbf{(Not Necessary?)}}}}

\label{subsec:systemv}

Following the daemon-agent framework, data appeared in an agent given by upper systems can not be directly accessed by daemons, since they belong to different processes with no common memory space, as shown in Section~\ref{subsec:RuntimeIsolation}.
Also, traditional inter-process communication approaches trigger extra data transfers, and significantly degrade the overall system performance.

To tackle this, we resort to kernel functions aided by UNIX System V. There is no extra memory overhead taken for daemons or agents to handle the data transferring.
Instead, a daemon has a unique System V key, that represents a specific System V share memory space in a local distributed node, while an agent has multiple keys to communicate with all daemons attached to the agent.
Agents and daemons can communicate with corresponding System V message queues, facilitating the sequence control of the system.
Also, 
% since data from upper systems or accelerators is kept in the System V share memory, 
{\color{blue}any data updates between agent and daemons can be immediately perceived by the other side, without extra sensing efforts or intermediate transfers, yielding the minimum data transferring between the two ends.}
%{
%\color{red}
%\textbf{(R4Q2)}
%}
%{
%\color{blue}
%Thus, as shown in Figure~\ref{fig:EXP_MidCost}, costs bought by middleware never change no matter the amount of existing deamon-agent framework, and the scalability of integrated system will be only determined by upper system.
%}
Furthermore, pipeline shuffle as shown in Section~\ref{subsec:pipelineShuffle}), can be implemented by changing the order of internal pointers of System V space. Such changes can also be observed by agents for subsequent memory operations, without any extra communication with daemons.

% Furthermore, System V IPC uses a series of user-specific keys to refer to different system V shared memory space and message queues. An agent can have multiple keys, indicating the connections with different daemons.
% During the runtime, daemons of a distributed node use keys in a pre-configured key set to generate different system V shared memory space and message queues, while the agent of the distributed node holds the whole key set. Then, the communication between daemon and agent is done with system V IPC.
%and access different daemons by passing corresponding keys to system V IPC.
%This mechanism supports daemon-agent based distributed system deployment, and makes our middleware can be applied on more specific system environments.

% Following the example used in Section \ref{subsubsec:MultiworkImp}, in a distributed node, multiple daemons, which represent multiple computation resources, can take part in the same computation task, with the help of the agent located in the same node. The agent and daemons communicate with data and msgs through the same System V space, and different System V keys are used to identify the connection with each other. 
