# Supplementary material for: GX-Plug: a Middleware for Plugging Accelerators to Distributed Graph Processing
Source: arXiv:2203.13005 source file (2022-03-31)
Supplement: Supplementary file 2 [file Appendix.tex]

\input{Appendix/Appendix_CodeExample.tex} 
